# Supplementary material for: Hypergraph Vision Transformers: Images are More than Nodes, More than Edges
Source: arXiv:2504.08710 source file (2025-04-11)
Supplement: Supplementary file 1 [file hypergraph_quality_notes.tex]

\section{Hypergraph Quality Notes}
\label{app:graph_quality}
We compute four metrics.

\subsection{Feature Entropy (Within Clusters)}

This measures the concentration of vertex features within each cluster (hyperedge). The idea is to quantify how "focused" the features in each hyperedge cluster are, by looking at the distribution of similarities between vertex features and the pooled feature for that hyperedge.

For each hyperedge $j$, calculate the cosine similarity between each vertex feature $V_i$ and the pooled hyperede feature given the incidence matrix $\mathbf{H}\in\mathbb{R}^{|V|\times|E|}$.
\begin{equation}
    E_{\mathrm{pool},j} = \frac{\sum_{i\in V} \mathbf{H}_{ij} V_i}{\sum_{i\in V} \mathbf{H}_{ij}}
\end{equation}

\begin{equation}
    \mathrm{cosine\_sim}(V_i, E_{\mathrm{pool},j}) = \frac{V_i \cdot E_{\mathrm{pool},j}}{||V_i|| \; ||E_{\mathrm{pool},j}||}
\end{equation}

Convert these probabilities into a probability distribution using the softmax function:

\begin{equation}
    p_{ij} = \frac{\mathrm{exp}\left(\mathrm{cosine\_sim}(V_i, E_{\mathrm{pool},j})\right)}
    {\sum_{\nu\in E_j}\mathrm{exp}\left(\mathrm{cosine\_sim}(V_\nu, E_{\mathrm{pool},j})\right)}
\end{equation}

Finally, calculate the entropy for the hyperedge $j$ as:

\begin{equation}
    H_j = -\sum_{i\in E_j} p_{ij} \; \mathrm{log}(p_{ij})
\end{equation}

This provides an entropy distribution over $|E|$ hyperedges. To measure the difference in distributions, we can use a KS test, or student's t-Test if the distributions are roughly normal.

This gives the entropy of the vertex feature distribution within the hyperedge cluster. Lower entropy indicates that the features are more concentrated (better intra-cluster coherence), and higher entropy means the features are more spread out (less coherence).

\begin{itemize}
    \item Kolmogorov-Smirnov (KS) Test: Compares two distributions and tells you if there’s a significant difference between them at any point. However, it doesn’t necessarily tell you directionality (i.e., whether one distribution is greater than the other).
    \item Lilliefors Test: This is a modification of the KS test designed for testing normality when the mean and variance are estimated from the sample. If you're checking whether your data is normally distributed (e.g., before using a parametric test like the t-test), Lilliefors would be helpful.
    \item One-Sided t-Test (if normality holds): If you check for normality (using the Shapiro-Wilk test or Lilliefors test) and the distributions are approximately normal, a one-sided t-test would be ideal for testing if one distribution has a significantly higher mean than the other. Null Hypothesis (H0) means of the two distributions are the same. Alternative Hypothesis (H1)  mean of one distribution is significantly greater than the other.
    \item Mann-Whitney U Test (if not normally distributed): The Mann-Whitney U test is a non-parametric alternative to the t-test. It’s great when the sample size is small, and it doesn’t assume normality. It tests whether one distribution tends to have larger values than the other. Null Hypothesis (H0) distributions are the same. Alternative Hypothesis (H1) one distribution tends to have higher values than the other.
\end{itemize}

\subsection{Intra-cluster Cosine Similarity}

This measures how similar the vertex features are within each cluster (hyperedge). The goal here is to compute the average cosine similarity between all vertices within a hyperedge, or between vertices and the pooled feature, giving a sense of how cohesive the features are within each cluster.

Compute the Vertex-to-Centroid Similarity: For each hyperedge $j$, calculate the similarity between each vertex feature $V_i$ and the pooled hyperedge feature $E_{\mathrm{pool},j}$. Then average these similarities to get the intra-cluster cosine-similarity for each hyperdege

\begin{equation}
    \mathrm{ACS}_j = \frac{1}{|E_j|}\sum_{i\in E_j} \mathrm{cosine\_sim}(V_i, E_{\mathrm{pool},j})
\end{equation}

This gives you a measure of intra-cluster cohesion based on the vertex-to-vertex or vertex-to-centroid similarity.

\subsection{Inter-cluster Distance}

This measures how distinct different clusters (hyperedges) are from one another. Specifically, it quantifies how far apart the pooled features $E_{\mathrm{pool},j}$ for different hyperedges are in feature space, using cosine distance.

For each pair of hyperedges $(j,k)$, compute the cosine distance between their pooled features $E_{\mathrm{pool},j}$ and $E_{\mathrm{pool},k}$.

\begin{equation}
    \mathrm{cosine\_distance}(E_{\mathrm{pool},j},E_{\mathrm{pool},k}) = 1 - \frac{E_{\mathrm{pool},j} \cdot E_{\mathrm{pool},k}}{||E_{\mathrm{pool},j}||\; ||E_{\mathrm{pool},k}||}
\end{equation}

Then average the distance ofr all pairs of hyperedges:

\begin{equation}
    AICD = \frac{1}{|E|^2} \sum_{j,k\in E} \mathrm{cosine\_distance}(E_{\mathrm{pool},j},E_{\mathrm{pool},k})
\end{equation}

This metric tells you how well-separated different clusters are. Higher inter-cluster distance means the hyperedges are grouping distinct features, indicating better cluster separation.

\subsection{Silhouette Score (for Cluster Quality)}

The Silhouette Score combines both intra-cluster similarity (how tight each cluster is) and inter-cluster distance (how well-separated clusters are). It gives an overall measure of the quality of the clustering.

Intra-cluster distance for vertex $V_i$ is the weighted average distance between $V_i$ and other vertices in the same hyperedge $E_j$:

\begin{equation}
    a(i, j) = \frac{\sum_{k\in V, k\neq i} \mathbf{H}_{kj}\; \mathrm{cosine\_distance}(V_i, V_k)}{\sum_{k\in V, k\neq i} \mathbf{H}_{kj}}
\end{equation}

Inter-cluster distance for vertex $V_i$ is the  minimum weighted distance between $V_i$ and the pooled feature of the nearest other hyperedge $E_k$:

\begin{equation}
    b(i,j) = \min_{k, k\neq j}\frac{\sum_m \mathbf{H}_{mk} \; \mathrm{cosine\_distance}(V_i, V_m)}{\sum_m \mathbf{H}_{mk}}
\end{equation}

The Silhouette Score for each vertex $V_i$ and hyperedge $E_j$ is then:

\begin{equation}
    s(i, j) = \frac{b(i,j) - a(i,j)}{\max(a(i,j), b(i,j))}
\end{equation}

This score indicates how well vertex $V_i$ is assigned to hyperdge $E_j$, relative to the nearest other hyperdge. The scores range between:

\begin{itemize}
    \item +1: The vertex is well-clustered.
    \item 0: The vertex is on the boundary between clusters.
    \item -1: The vertex is closer to another hyperedge than its own.
\end{itemize}

The aggregate Silhouette Score is then:

\begin{equation}
    S(\mathcal{G}) = \frac{1}{|V|}\sum_{i\in V} \frac{\sum_{j\in E} \mathbf{H}_{ij}\; s(i,j)}{\sum_{j\in E} \mathbf{H}_{ij}}
\end{equation}

The global Silhouette Score for the graph is a single value that provides a measure of how well-clustered the entire graph is, based on the intra-cluster cohesion and inter-cluster separation of vertices with respect to the hyperedges they belong to.

\begin{itemize}
    \item Positive values (closer to +1) suggest that the hypergraph model is performing well, with well-separated and cohesive clusters.
    \item Scores close to 0 suggest that the hypergraph’s clustering is ambiguous and may need improvement (e.g., hyperedges could be overlapping, or vertex memberships may not be well-defined)
    \item Negative values (closer to -1) indicate that the clustering is poor, and the hypergraph’s structure may not effectively represent the relationships between vertices and hyperedges.
\end{itemize}

When comparing models, the higher the global Silhouette Score, the better the clustering quality. The interpretetation in sets (DINO, VGNN) = (D,V) and poolin (Image, Edge) = (I,E).

\begin{itemize}
    \item (D, I) > (V, I): DINO features perform better than VGNN features when using image pooling, suggesting that DINO embeddings capture higher-level semantic information compared to VGNN, which may focus on textures.
    \item (V, E) > (V, I): Edge pooling outperforms image pooling using VGNN features, meaning that edge pooling encourages more structured, semantically meaningful clustering, possibly mitigating VGNN's focus on low-level texture features.
    \item (D, E) > (V, E) happens, it would mean that DINO features still outperform VGNN features even when edge pooling is applied, indicating that DINO's superior semantic representation continues to enhance clustering. Edge pooling, VGNN features still suffer from their focus on low-level visual characteristics (like textures).
    \item  (D, E) > (D, I) this means that DINO features perform better with edge pooling than with image pooling. Since DINO features are known to capture higher-level semantic information, this outcome indicates that edge pooling is more effective at capturing and utilizing the semantic relationships within the DINO embedding space than image pooling.
    \item (D, E) > (D, I) and (V, I) > (V, E) Edge pooling is more effective at organizing semantic information when using DINO features. This means that the relationships between vertices (as defined by the hypergraph) are semantically meaningful when pooled at the hyperedge level. In contrast, VGNN’s image pooling is better at clustering based on low-level visual properties, such as textures. Since image pooling groups features from local image patches, it’s more likely to preserve visual patterns (like textures, edges, etc.) that VGNN features excel at capturing.
\end{itemize}

\FloatBarrier
